# Supplementary material for: Permutation Invariant Policy Optimization for Mean-Field Multi-Agent Reinforcement Learning: A Principled Approach
Source: arXiv:2105.08268 source file (2021-05-18)
Supplement: Supplementary file 1 [file appendix_experiment.tex]

%!TEX root = marl.tex

% \appendix

\section{Experimental details}
\label{app:experiment}
